# Supplementary material for: Measuring and Controlling Solution Degeneracy across Task-Trained Recurrent Neural Networks
Source: arXiv:2410.03972 source file (2025-11-20)

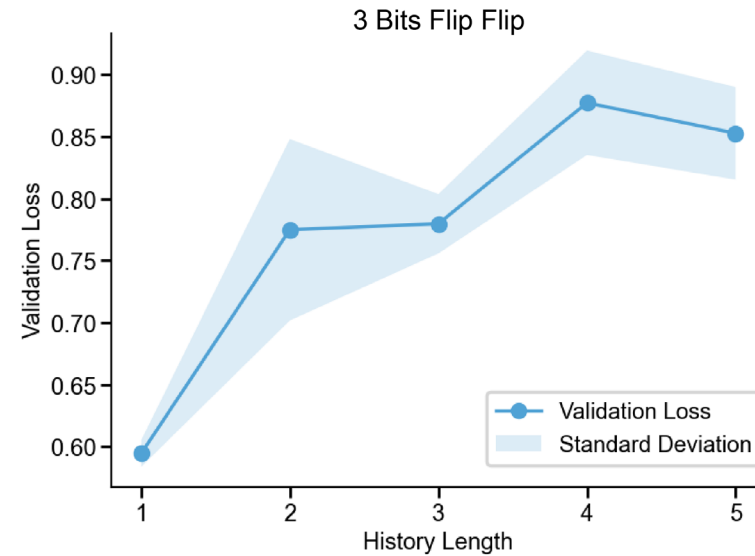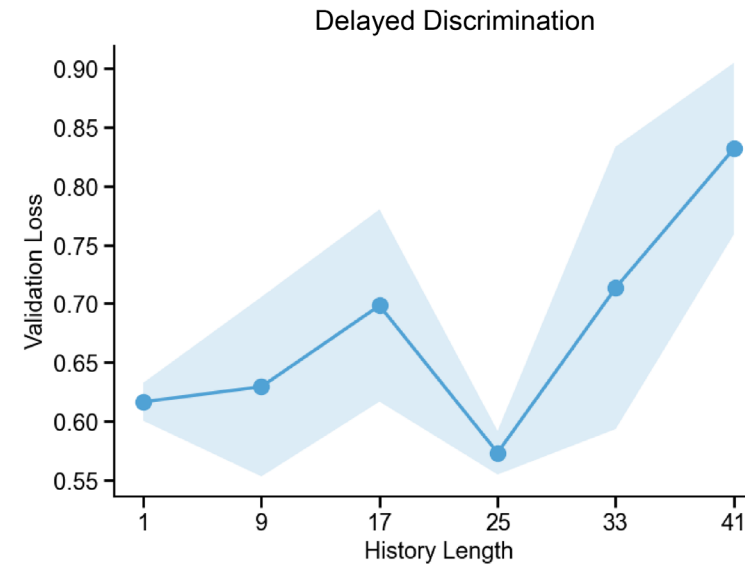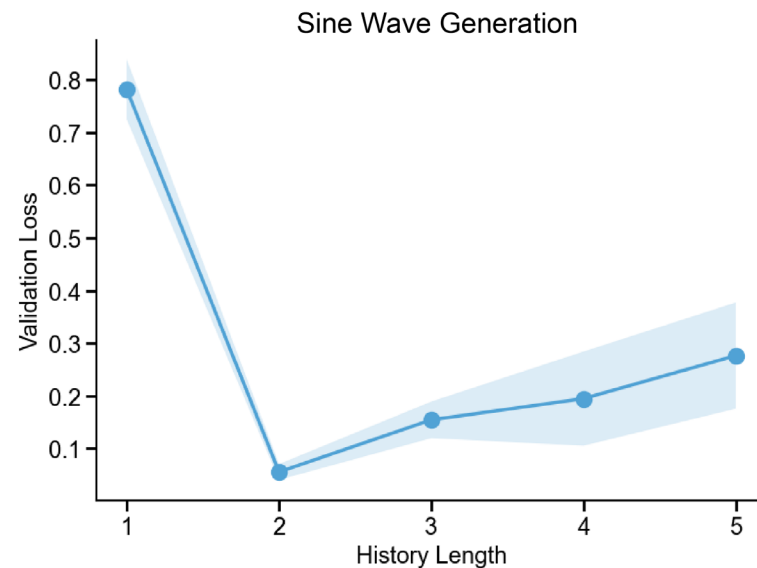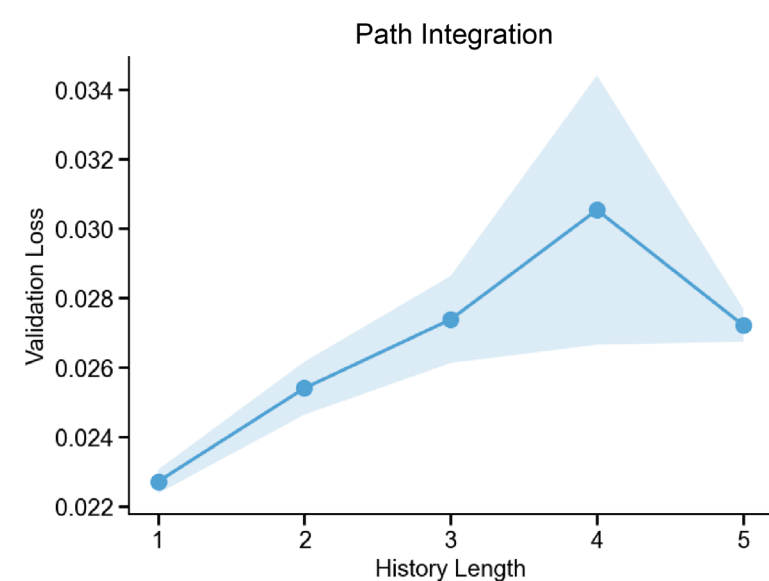

## Task Complexity

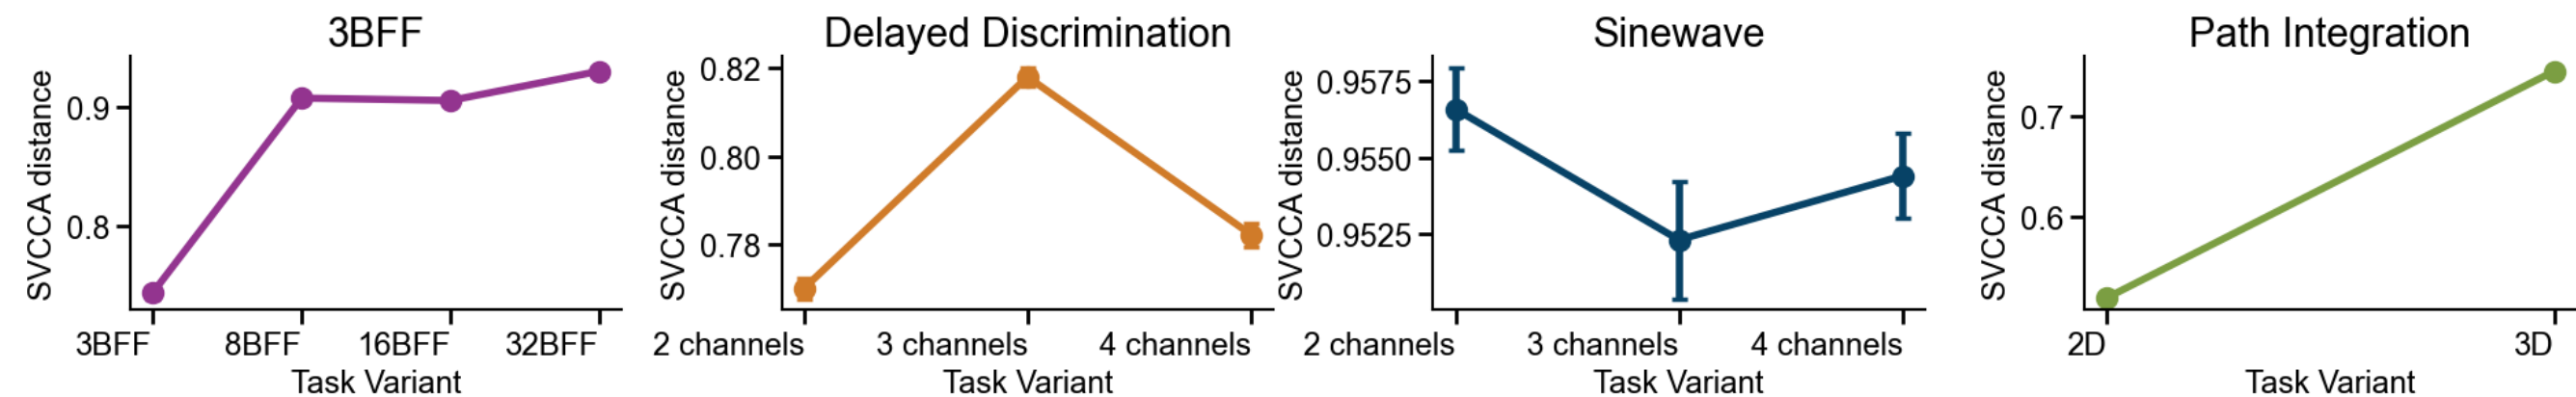

## Feature Learning

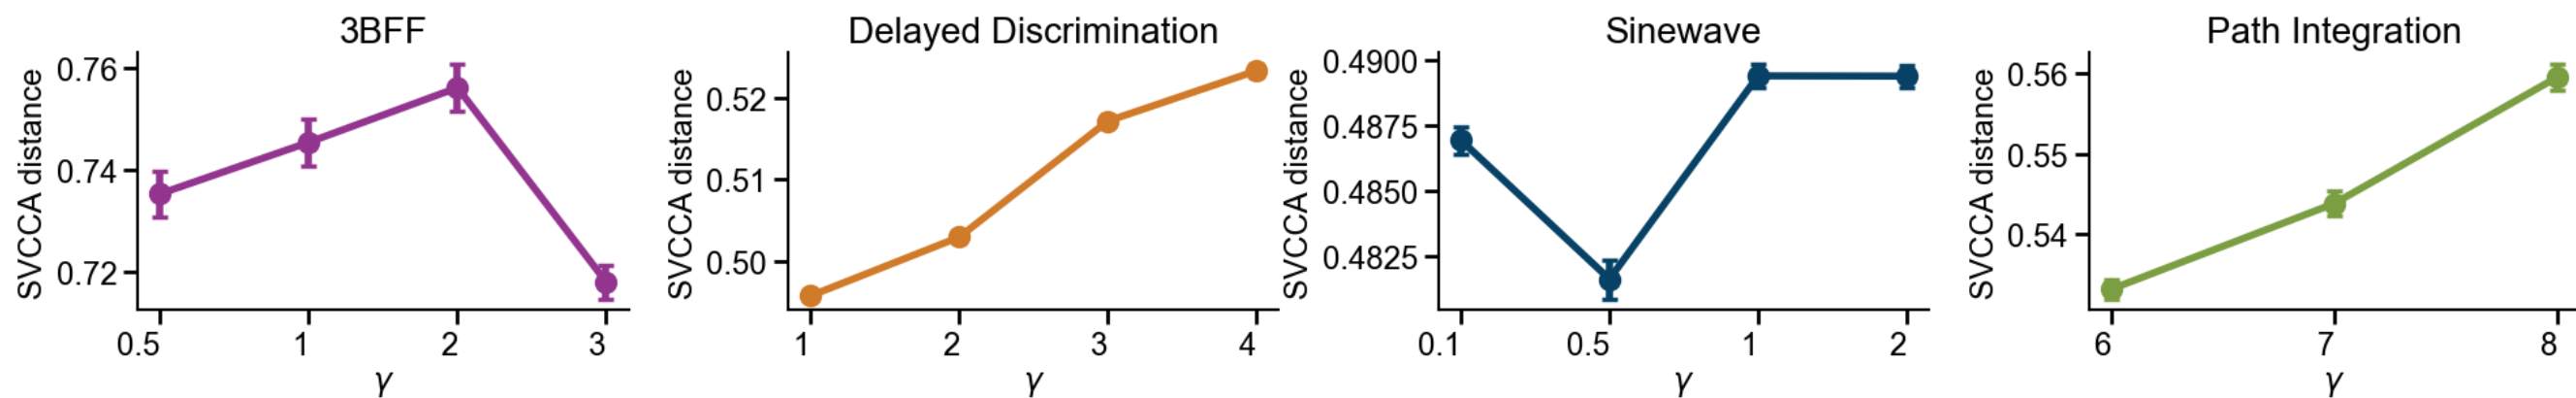

## Network Size

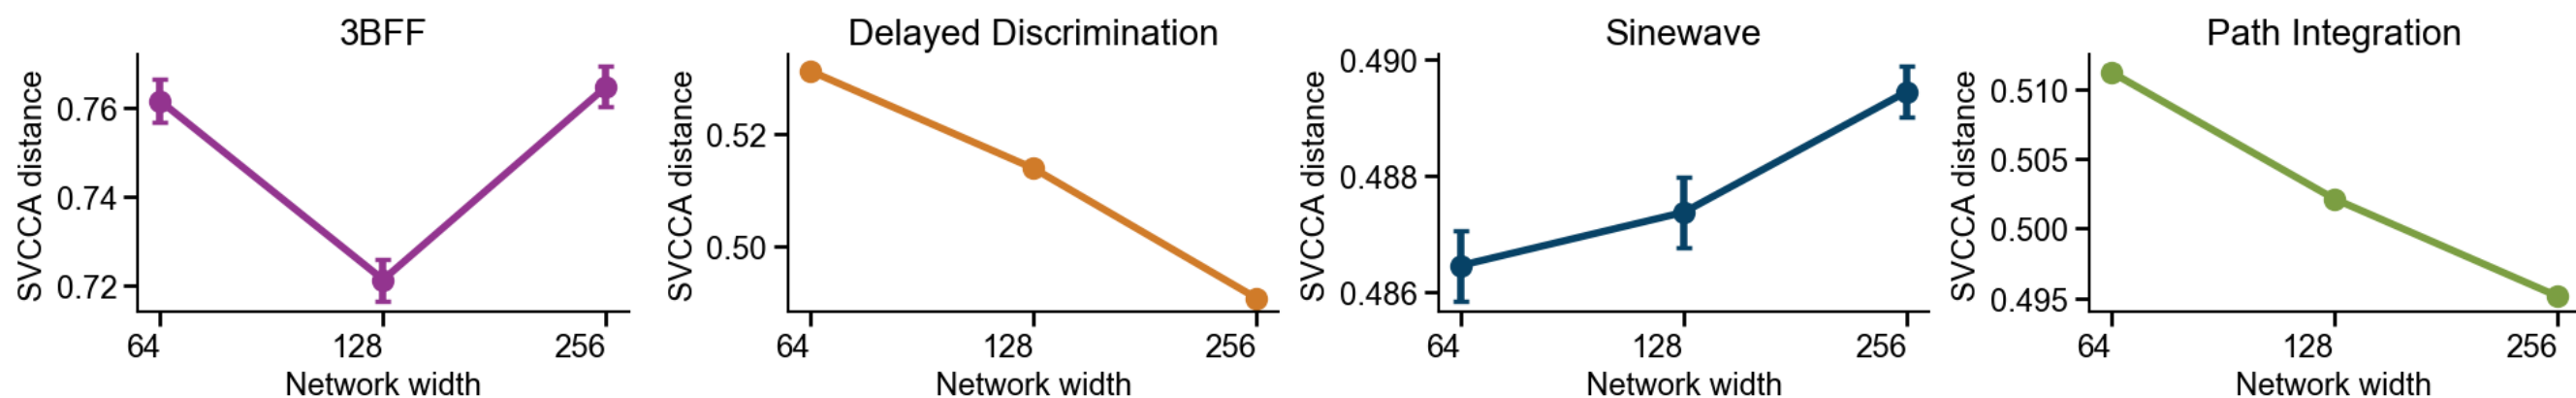

## Regularization on Delayed Discrimination

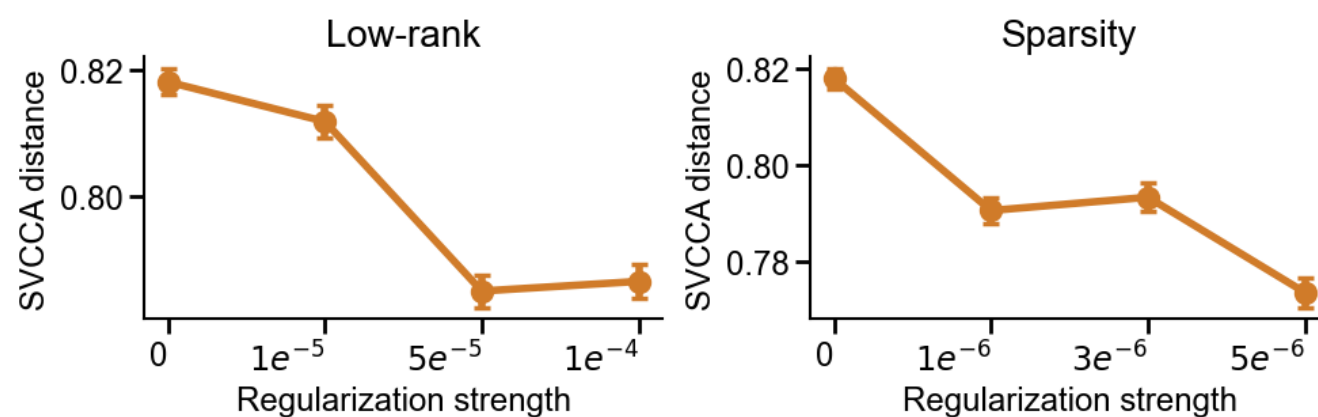

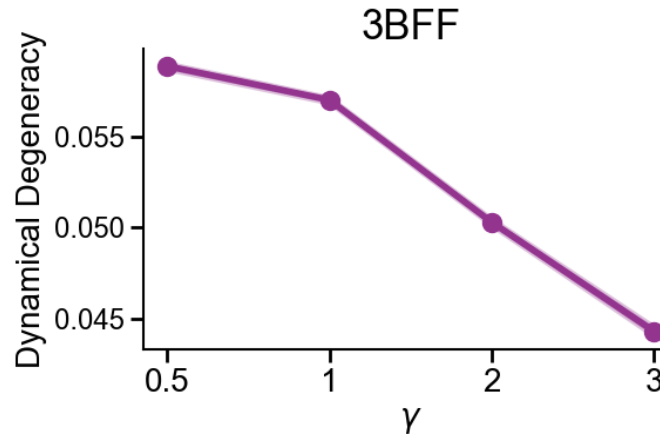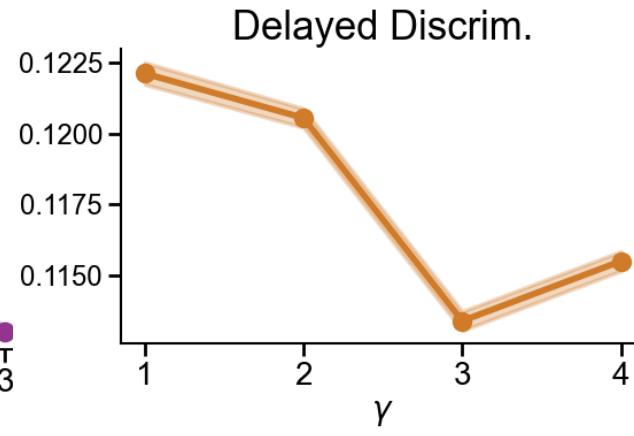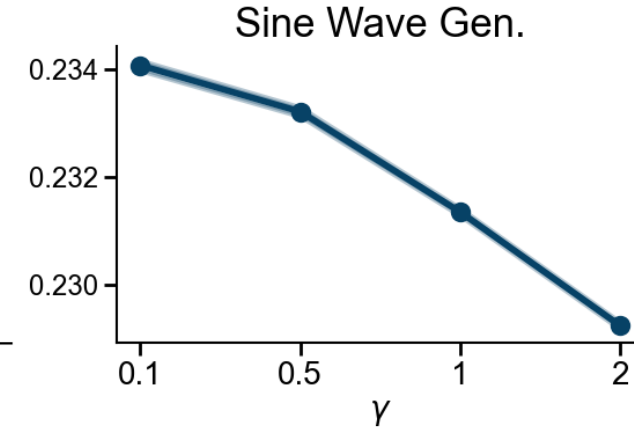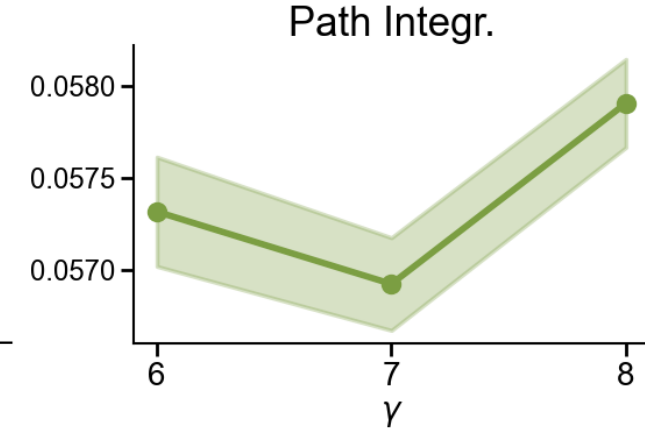

Supplement: Supplementary file 1 [file memory_demand.pdf]
